# Supplementary material for: Sparse Ellipsometry: Portable Acquisition of Polarimetric SVBRDF and Shape with Unstructured Flash Photography
Source: arXiv:2207.04236 source file (2023-02-08)
Supplement: Supplementary file 1 [file appendix.tex]

\section*{Appendix}
\label{sec:appendix}
Notations are summarized in Table~\ref{tab:notations}.
\input{notations}
